# Supplementary material for: MAG$\pi$: Types for Failure-Prone Communication
Source: arXiv:2301.10827 source file (2023-01-25)
Supplement: Supplementary file 1 [file pingpong.tex]

We show the processes and properties of the ping pong example from the introduction.

\footnotesize{\begin{align*}
        \begin{array}{c}
            \contG = \{\cSessionRole{s}{p}:\tSession_\role{p},\ \cSessionRole{s}{q}:\tSession_\role{q}, \cSessionRole{s}{r}:\tSession_\role{r}\}
            \\[1em]
            P_{\textit{ping}} = \cRestriction{s:\contG}{\ \cPar{P_\role{p}\ }{\ \cPar{P_\role{q}\ }{\ \cPar{P_\role{r}\ }{\ \cBuffer{s}{\emptyBuffer}}}}}
            \\[1em]
            P_\role{p} = \cSnd{\cSessionRole{s}{p}}{q}{ping}{}{
                \cBranchL{\cSessionRole{s}{p}}{
                    \begin{array}{l}
                        \cRcv{q}{pong}{}{P_\role{p}^\textit{ok}}, \\
                        \cTimeOut{\cSnd{\cSessionRole{s}{p}}{q}{ping}{}{
                            \cBranchL{\cSessionRole{s}{p}}{
                                \begin{array}{l}
                                    \cRcv{q}{pong}{}{P_\role{p}^\textit{ok}}, \\
                                    \cTimeOut{\cSnd{\cSessionRole{s}{p}}{q}{ping}{}{
                                        P^\prime_\role{p}
                                    }}
                                \end{array}
                            }
                        }}
                    \end{array}
                }
            }
            \\[2em]
            P_\role{p}^\textit{ok} = \cSnd{\cSessionRole{s}{p}}{r}{ok}{}{\inaction}
            \Sep
            P_\role{p}^\prime = \cBranchL{\cSessionRole{s}{p}}{
                \begin{array}{l}
                    \cRcv{q}{pong}{}{P_\role{p}^\textit{ok}}, \\
                    \cTimeOut{\cSnd{\cSessionRole{s}{p}}{r}{ko}{}{\inaction}}
                \end{array}
            }
            \\[2em]
            P_\role{q} = \cBranchL{\cSessionRole{s}{q}}{
                \begin{array}{l}
                    \cRcv{p}{ping}{}{P_\role{q}^\textit{pong}},\\
                    \cTimeOut{\cBranchL{\cSessionRole{s}{q}}{
                        \begin{array}{l}
                            \cRcv{p}{ping}{}{P_\role{q}^\textit{pong}}, \\
                            \cTimeOut{\cBranch{\cSessionRole{s}{q}}{
                                \cRcv{p}{ping}{}{P_\role{q}^\textit{pong}},\ 
                                \cTimeOut{\inaction}
                            }}
                        \end{array}
                    }}
                \end{array}
            }
            \\[2em]
            P_\role{q}^\textit{pong} = \cSnd{\cSessionRole{s}{q}}{p}{pong}{}{\inaction}
            \\[1em]
            P_\role{r} = \cBranch{\cSessionRole{s}{r}}{\cRcv{p}{ok}{}{\inaction}, \cRcv{p}{ko}{}{\inaction}}
        \end{array}
    \end{align*}}

\subsubsection{Properties} Since we have $(\{s\};\rel)$-\emph{bound}$_4(\contG)$, by 
\cref{thm:decidable-props} it holds that determining \emph{safety}, 
\emph{deadlock-freedom}, \etc\ is decidable for \contG. 
Upon inspection of \contG, we find that $(\{s\};\rel)$-$\phi(\contG)$ for 
$\phi \in $ \{\emph{safe}, \emph{deadlock-free}, \emph{terminating}, \emph{live}\}.
